# Supplementary material for: A Review of the Deep Sea Treasure problem as a Multi-Objective Reinforcement Learning Benchmark
Source: arXiv:2110.06742 ancillary file (2024-05-21)
Supplement: Supplementary file 1 [file supplement.pdf]

## 1 Configurations

The configuration that the authors used for the bi-objective Deep Sea Treasure (DST) can be found in the supplementary materials in `2-objective-config.json`, and the configuration that was used for the tri-objective DST can be found in `3-objective-config.json`.

## 2 Missing Proofs

### 2.1 Bi-Objective

Following [Rădulescu et al., 2019], we will use the discounted reward for all proofs, in the knowledge that for finite-horizon Markov Decision Processes (MDPs) like ours,  $\gamma$  can be taken as 1:

$$G_t \doteq R_{t+1} + \gamma \cdot R_{t+2} + \gamma^2 \cdot R_{t+3} + \dots = \sum_{k=0}^N \gamma^k R_{t+k+1} \quad (1)$$

We will attempt to prove properties regardless of which value is chosen for  $\gamma$ , although sometimes exceptions might have to be made for edge cases.

Before deriving the properties of the DST environment, we will first define a number of conventions and assumptions made throughout the paper and these proofs

- a All treasures values are  $> 0$
- b  $0 < \gamma \leq 1$  (The exclusion of  $\gamma = 0$  will be justified at the end of section 2.1.2 and section 2.2.2)
- c The MDP we use is a finite-horizon MDP ending after 1000 environment interactions.
- d The starting square for the environment  $(0, 0)$  does not contain any treasure.

#### 2.1.1 Collisions

In the original DST problem, agents are capable of causing collisions by attempting to move out of the world. In this section, we will prove that any sequence of actions containing a collision is Pareto-dominated by one or more other sequence(s) of actions. Due to the nature of the DST problem described in our paper, a collision due to  $a_t$  has the following properties:

- The environment state is not altered
- The immediate time reward for a collision is not altered
- The immediate treasure reward for a collision is 0

Or more formally:

- $s_t = s_{t+1}$
- $r_b(s_t, a_t) = -1$
- $r_p(s_t, a_t) = 0$

*Proof.* We define an episode  $E$  that has reached a terminal state after  $T$  time steps.  $E$  will consist of a sequence of state, action, next state and reward tuples.

$$E = \{(s_0, a_0, s_1, \mathcal{R}(s_0, a_0)), \dots, (s_T, a_T, \emptyset, \mathcal{R}(s_T, a_T))\} \quad (2)$$

This yields a total, discounted reward of:

$$G_T = \left( - \sum_{j=0}^T \gamma^j, r_p(s_T, a_T) \cdot \gamma^T \right) \quad (3)$$

We will now assume that  $a_i$  caused a collision. Our intention is to simply remove  $(s_i, a_i, s_{i+1}, \mathcal{R}(s_i, a_i))$  from  $E$  without causing a change in  $s_{i+1}, a_{i+1}$ .

Thanks to the Markov Property [Sutton and Barto, 1998] and the fact that our policy  $\pi$  only depends on the current state if  $s_{i+1}$  stays the same, we can assume that  $s_T$  also stays the same, resulting in our agent finding the same solution:

$$s_{i+1} = s'_{i+1} \quad (4)$$

$$\implies s_T = s'_T \quad (5)$$

Using the definition of our dynamics, we know that, in the case of collision,  $s_{i+1} = s_i$ , this satisfies the conditions we set out earlier, and allows us to continue our analysis under the assumption that our solution remains unchanged.

$$E' = E \setminus (s_i, a_i, s_{i+1}, \mathcal{R}(s_i, a_i)) \quad (6)$$

After removing  $a_i$  from  $E$ , we will analyze the total discounted reward, to determine the effect on the Pareto-optimality of the solution we found. Since  $E'$  contains 1 less tuple than  $E$ , the time-reward will have changed, but since we still found the same treasure, our treasure reward remains unchanged:

$$G'_T = \left( \left( - \sum_{j=0}^{T-1} \gamma^j \right), r_p(s_T, a_T) \cdot \gamma^T \right) \quad (7)$$

Since

$$0 < \gamma \leq 1 \implies - \sum_{j=0}^T \gamma^j < \left( - \sum_{j=0}^{T-1} \gamma^j \right) \quad (8)$$

It follows that the solution found by  $E'$  weakly-Pareto-dominates  $E$  (In this paper, we will denote solution  $a$  being dominated by solution  $b$  as  $a \prec b$ ):

$$E \prec E' \quad (9)$$

■

Through this proof, we have shown that a trajectory containing a collision is always Pareto-dominated by the same trajectory, but with the collision removed. We have done so without making any assumptions about the actual trajectory, besides the fact that it contains a collision.

### 2.1.2 Time-Outs

An episode in the DST problem can end one of two ways:

1. The agent takes the maximum number of steps (1000)
2. The agent finds a treasure

In this section, we will only consider the first situation, showing that any solution that ends in this way is sub-optimal, and thus can be disregarded when searching for optimal solutions to the DST problem.

*Proof.* We first define an episode  $E$ , as a set of state, action, next state and reward tuples.  $s_N$  is assumed to be non-terminal, while  $a_N$  is assumed to terminate  $E$ .

$$E = \{(s_0, a_0, s_1, \mathcal{R}(s_0, a_0)), \dots, (s_{N-1}, a_{N-1}, s_N, \mathcal{R}(s_{N-1}, a_{N-1}))\} \quad (10)$$

Since the agent is not in a terminal state, it hasn't found a treasure yet, from this, we can derive

$$\forall i \in \{0, \dots, N-1\} : \mathcal{R}(s_i, a_i) = (-1, 0) \quad (11)$$

From this point on, there are two options, either we find a treasure with value  $t$  on the next step, or we don't. Our cumulative reward after  $N$  steps can thus be described as:

$$G_N = \begin{cases} \left(-\sum_{i=0}^N \gamma^i, 0\right) & \text{if } 0 = r_p(s_N, a_N) \\ \left(-\sum_{i=0}^N \gamma^i, p \cdot \gamma^N\right) & \text{if } 0 \neq r_p(s_N, a_N) \end{cases} \quad (12)$$

Since (See 2.1)

$$0 < p \text{ and } 0 \leq \gamma \leq 1 \quad (13)$$

$$\implies 0 \cdot \gamma^N \leq p \cdot \gamma^N \quad (14)$$

$$\implies 0 \leq p \cdot \gamma^N \quad (15)$$

From this, it follows that a solution that ends in the agent not finding treasure, is always weakly-Pareto-dominated by any solution that does find a treasure, as long as  $0 < \gamma$ :

$$\forall p \in \mathbb{R}_0^+ : \left(-\sum_{i=0}^N \gamma^i, 0\right) \prec \left(-\sum_{i=0}^N \gamma^i, p \cdot \gamma^N\right) \quad (16)$$

In this equation, we'd like to point out that both episodes are assumed to be of equal length, with 1 ending in a time-out, while the other ends in finding treasure. While this is enough to prove what we set out to prove, we also note that a solution that takes the maximum possible number of steps to reach a treasure will usually be dominated by a solution taking a more direct route. ■

If  $\gamma = 0$ , the total reward of any episode is  $G = (-1, r_p(s_0, a_0))$ . Since the time-objective is equal in all cases, the Pareto-front will consist of a single point, corresponding to finding the treasure directly below the agent in a single action. We note that this is only true when using the default shape for the seabed, if treasures are placed in other locations, the Pareto-front might shift, however, since only the treasure-objective is relevant, the Pareto-front will never consist of more than 1 point, even if multiple treasures can be reached. In this case, the Pareto-front will only contain the solution with the highest treasure value. If no treasures can be reached in a single action, the Pareto-front will only contain the solution  $G = (-1, 0)$ .

In this section, we have thus proven that any solution which ends in a time-out can be discarded when searching for optimal solutions to the DST problem.

## 2.2 Tri-Objective

### 2.2.1 Collisions

In this section, we will review the proof on collisions from section 2.1.1. We note that, in addition to the properties of collisions already listed in section 2.1.1, the tri-objective environment also has one more property related to its fuel objective:

- The fuel objective is 0 when colliding

Formally:

- $r_f(s_t, a_t) = 0$  when colliding

To facilitate this review, we also need to re-formulate our definition of a collision. In the tri-objective environment, it is possible for an agent to accumulate more velocity than it can arrest in a single timestep. Because of this, we will define a collision as a set of multiple, consecutive timesteps, leading to a collision, that could have prevented this collision. More formally, if we define an episode  $E$  as follows:

$$E = \{(s_0, a_0, s_1, \mathcal{R}(s_0, a_0)), \dots, (s_T, a_T, \emptyset, \mathcal{R}(s_T, a_T))\} \quad (17)$$

In episode  $E$ , we define a subsequence of timesteps  $C_{i,j}$  that cause a collision:

$$C_{i,j} = \{(s_i, a_i, s_{i+1}, \mathcal{R}(s_i, a_i)), \dots, (s_j, a_j, s_{j+1}, \mathcal{R}(s_j, a_j))\} \quad (18)$$

At this point, we would have to modify  $a_i$  through  $a_j$  in such a way that they prevent a collision. Following this,  $s_{j+1}$  would be different from its original value, since the agent will end up in different location with a different velocity because of the modifications to  $a_i$  through  $a_j$ . In turn, this would make it impossible to say anything about the optimality of the modified episode, mainly due to the formulation of the fuel objective.

While it may be possible to find a general formulation for this situation, the authors feel that the added necessary effort speaks to the higher complexity of the tri-objective environment, and that this shows that optimal solutions for this environment are likely much less trivial to find than those of the original environment.

### 2.2.2 Time-Outs

Next, we revisit the proof on time-outs made earlier in section 2.1.2, taking our fuel objective into account. In this proof, we will take a different approach, instead proving that there is at least 1 solution ending in a time-out, that is always part of the pareto-front, thus invalidating the claim that time-outs are always suboptimal in the tri-objective case.

*Proof.* For this proof, we will consider an agent with a preference for optimizing the fuel-objective first, and any other objectives second. The most optimal solution for this agent, would be a solution that consumes no fuel. Fuel consumption for an action  $a$  in state  $s$  is given by:

$$r_f(s, a) = -(a_x^2 + a_y^2) \quad (19)$$

When discounting and summing over an entire episode  $E$  consisting of  $T$  timesteps, this yields

$$G_{E,f} = - \sum_{i=0}^T \gamma^i \cdot (a_{x,i}^2 + a_{y,i}^2) \quad (20)$$

Since

$$\forall i \in \mathbb{N} : -\gamma^i \cdot (a_{x,i}^2 + a_{y,i}^2) \leq 0 \quad (21)$$

The most optimal policy with regard to fuel would use 0 fuel.

From the formulation in equation 20, it is clear that a policy that consumes 0 fuel is only possible under two circumstances:

1.  $\gamma = 0$
2.  $\forall i \in 0, \dots, T : a_{x,i} = 0 \wedge a_{y,i} = 0$

We will first consider the second situation, which follows from the fact that  $\forall x \in \mathbb{R} : 0 \leq x^2$ . In this situation both  $a_x$  and  $a_y$  are 0 for all actions. It is clear to see that this is possible in the tri-objective environment, from the formulation of the action space:  $\{-3, -2, \dots, 2, 3\}^2$ , by using action  $(0, 0)$ . We note that this is also the only action that would allow the total discounted fuel reward to be 0.

Finally, we will look at the solution that an agent finds by taking this action for every step of an episode. We can denote this episode as  $E$ :

$$E = \{(s_0, (0, 0), s_1, \mathcal{R}(s_0, (0, 0))), \dots, (s_T, (0, 0), \emptyset, \mathcal{R}(s_T, (0, 0)))\} \quad (22)$$

When looking at the environment dynamics, we can see that  $s_0 = s_T$ . Practically, this means that the agent never moves from its initial position. Since the agent can not start on a treasure, this implies that the only way to end an episode is through a time-out. Calculating the total discounted reward then gives us:

$$G_T = \left( - \sum_{i=0}^T \gamma^i, 0, 0 \right) \quad (23)$$

From this, it follows that there is only one solution resulting in a total discounted fuel reward of 0 (With  $0 < \gamma \leq 1$ ), and this solution is always part of the Pareto-front, since it is impossible to achieve a total discounted fuel reward  $> 0$ .

Finally, we review the result of considering  $\gamma = 0$ . In section 2.1.2, we showed that in the bi-objective case, this results in a Pareto-front containing only a single solution. In the tri-objective case, this is no longer true. The size of the Pareto-front in this case, will be equal to 1 + the number of treasures that can be reached in a single action, with a unique combination of fuel cost and treasure. The +1 is added, because the time-out solution is still valid, and optimal. ■

## References

- [Rădulescu et al., 2019] Rădulescu, R., Mannion, P., Roijers, D. M., and Nowé, A. (2019). Multi-objective multi-agent decision making: a utility-based analysis and survey. *Autonomous Agents and Multi-Agent Systems*, 34.
- [Sutton and Barto, 1998] Sutton, R. S. and Barto, A. G. (1998). *Reinforcement Learning An Introduction*. MIT Press, London.
